# Supplementary material for: Controlled propulsion and separation of helical particles at the nanoscale
Source: arXiv:1605.00768 source file (2017-01-30)
Supplement: Supplementary file 1 [file SI.pdf]

# Controlled propulsion and separation of helical particles at the nanoscale

Maria Michiko T. Alcanzare*[1], Vaibhav Thakore[1], Santtu T. T. Ollila[2], Mikko Karttunen[3], and Tapio Ala-Nissila[1,4]

[1]COMP CoE at the Department of Applied Physics, Aalto University School of Science, P.O. Box 11000, FIN-00076 Aalto, Espoo, Finland
[2]Varian Medical Systems Finland, Paciuksenkatu 21, 00270 Helsinki, Finland
[3]Department of Mathematics and Computer Science & Institute for Complex Molecular Systems, Eindhoven University of Technology, P.O.Box 513, MetaForum 5600 MB Netherlands
[4]Department of Physics, Brown University, Box 1843, 182 Hope Street Barus & Holley, Providence, Rhode Island 02912-1843, USA

December 21, 2016

## Rotational Reynolds Number

The rotational Reynolds number is calculated as

$$\mathrm{Re}_R = \frac{\rho D^2 \omega}{\eta} \tag{1}$$

where $\omega$, $D$, $\rho$ and $\eta$ are the angular velocity, helical diameter, fluid density and fluid viscosity, respectively. In Fig. S1, we show the variation of the rotational Reynolds number for different parameters. In our simulations it varies from $9 \times 10^{-3}$ to $2 \times 10^{-4}$.

*maria.alcanzare@aalto.fi

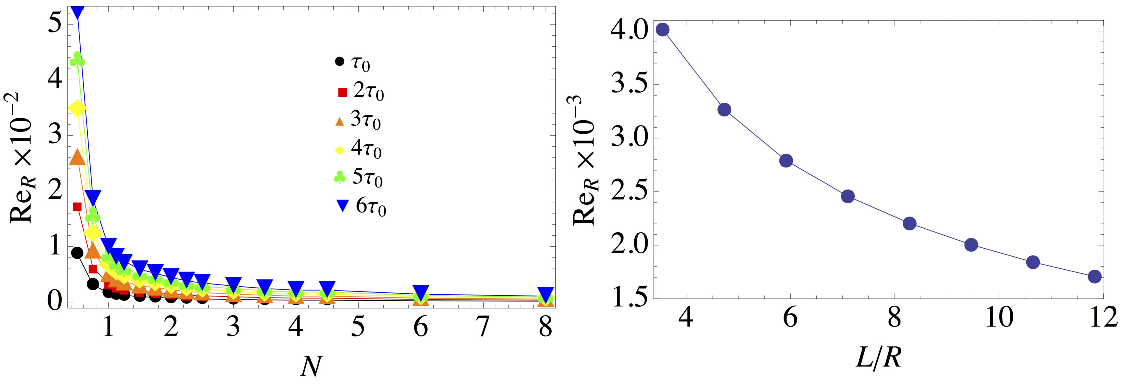


(a) (b)

Figure S1: Rotational Reynolds $\mathrm{Re}_R$ numbers (a) as a function of the number of turns for varying torque strengths for $L/R = 5.92$ and (b) as a function of pitch length and helical radius ratio for $N = 1.25$. Here, $\tau_0 = 1.0 \times 10^{-18}$ kg m$^2$/s$^2$

## Rotational drag coefficient

In Fig. S2, the rotational drag coefficients along the long axis of the helix are plotted as a function of the number of turns. The drag coefficients $\kappa_{\mathrm{rot}}$ were obtained from the simulations by taking the slope of the angular velocity of the helix as a function of the hydrodynamic drag along the long axis.

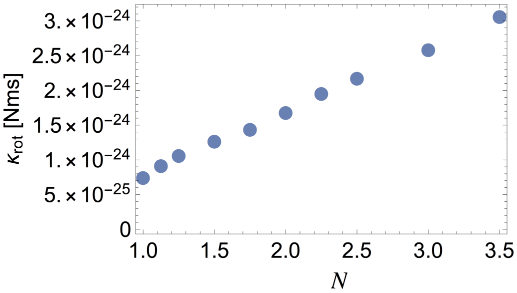


Figure S2: The viscous rotational drag coefficients along the long axis of the helix are plotted as a function of the number of turns for $L/R = 5.92$.

## Shape optimization

In the main text, the propulsion velocity and the efficiency are shown to depend on the geometrical shape of the helical particle (cf. Figs. 1 and 5). Here, for the propulsion of the helical particles with different areas of cross-section, namely the helix, helicoid A and helicoid B, it is shown that the helix has an optimal angular velocity because it experiences less viscous drag from its smaller surface area than the other two shapes (Fig. S3). Thus, the propulsion velocity is maximized for

the helix.

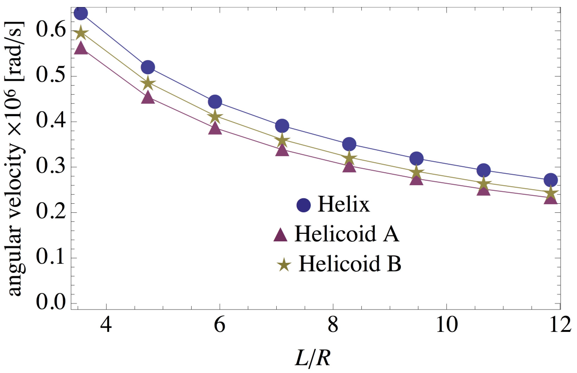


Figure S3: Angular velocities of the helix, helicoid A and helicoid B for pitch length and helical radius ratio of $L/R = 5.92$, and $N = 1.25$ helical turns. The data have been obtained without thermal fluctuations.

## Wobbling of the helices - influence of thermal fluctuations

In Fig. S4, the projection of the orientation of the long axes of the helices along their initial orientations is plotted against time for the Methods 1 and 2. When a constant torque (Method 1) is applied on the helical particles, strong wobbling is observed in the smaller helices with fractional turns ($N < 1$). This wobbling decreases with the increasing number of turns $N$ due to the increase in the symmetry of these helices (see Fig. S4 A). Thus, for large non-integer values of the helical turns wobbling is negligible and the helical particle moves in a straight line. The differences between the Methods 1 and 2 for the deterministic and the thermalized cases are illustrated in Fig. S4 B.

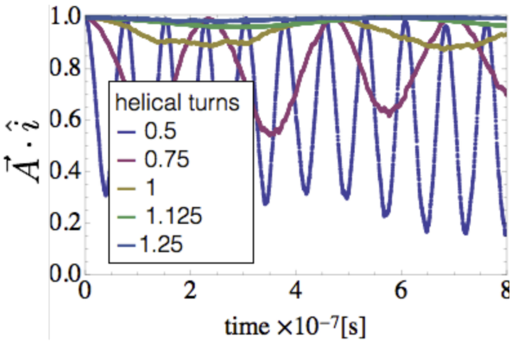


Figure S4: The projection of the long axis of the helix along $\hat{u}_x$ for different values of helical turns at constant external torque, without thermal fluctuations. Oscillations in the data indicate wobbling of the helices.

## Propulsion efficiency

In Fig. S5 we show the efficiencies $\epsilon = v/(\omega R)$ for the three different shapes as a function of the ratio $L/R$. In contrast to the data in Fig. 2.a for the propulsion velocities, the efficiency depends only weakly on the particle geometry and is maximized at a somewhat larger value of $L/R$ that the velocity (see also Fig. 2.c in the main text).

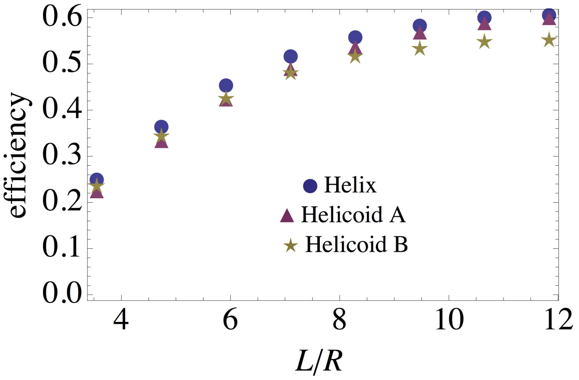


Figure S5: Efficiencies of the different helical particles as a function of the pitch length for $N = 1.25$ helical turns.

## Rotation with thermal fluctuations

The rotation due to the external torque applied on the helices overcomes the effects of the thermal fluctuations on the rotational motion of the helices. In SI Fig. S6, we observe that the perpendicular orientations are unaffected by the thermal fluctuations since $\tau > 48k_BT$.

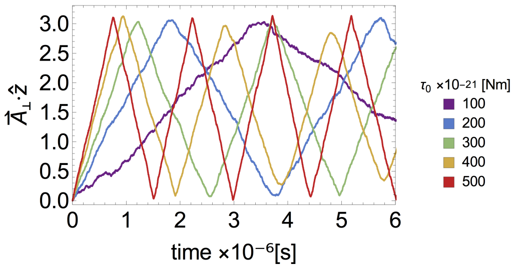


(a) $N = 0.5$

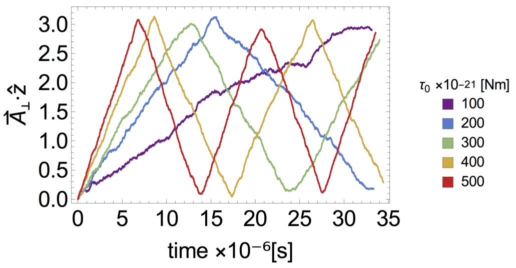


(b) $N = 1.25$

Figure S6: Plot shows the orientation of the perpendicular axis $\boldsymbol{A}_\perp \cdot \hat{z}$ at different torque strengths for $N = 1.25$ $L/R = 5.92$, with thermal fluctuations.

### Helical length

As expected, both the angular and propulsion velocities grow linearly with increasing torque. Once the helical particles have achieved stable motion for a given torque, the angular and the propulsion

velocities scale inversely with the number of turns $N$ of the helices for large values, as shown in Fig. S7.

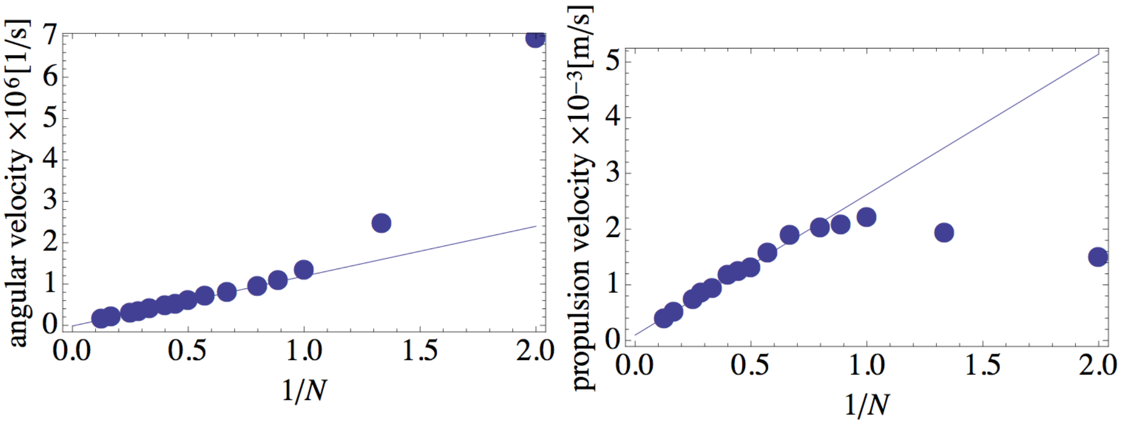


(a) (b)

Figure S7: (a) Deterministic angular and (b) propulsion velocities of a driven helix with $N$ helical turns, 30 nm helical radius, $L/R = 5.92$ pitch length to helical radius ratio, and $\tau = 1.0 \times 10^{-18}$ kg m$^2$/s$^2$ external torque. The continuous line is an asymptotic $1/N$ fit of the data.

## Fluidity

In the simulations without thermal fluctuations at low Reynolds numbers, the angular and the propulsion velocities obtained are consistent with linear dependence on the fluidity in the Stokes' limit, as shown in Fig. S8.

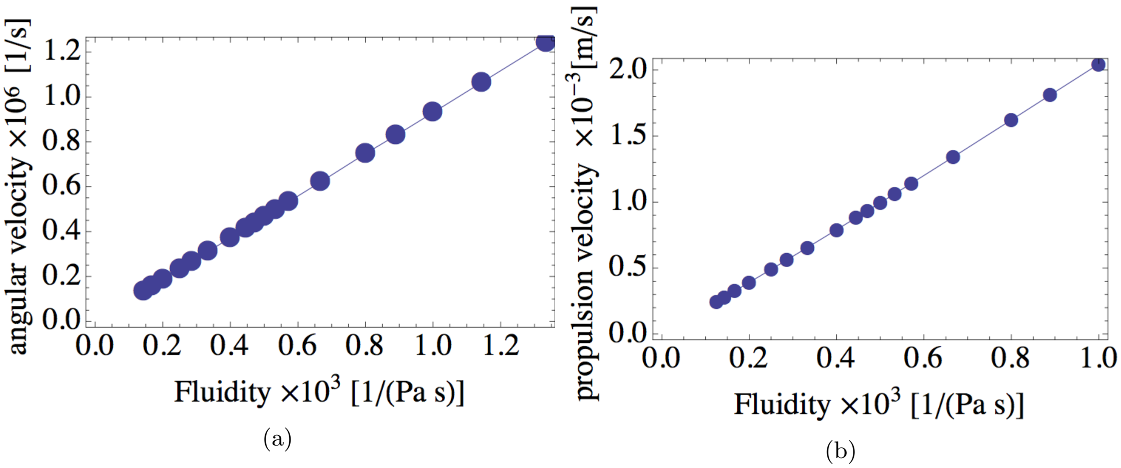


Figure S8: (a) Angular frequency and (b) propulsion velocity as a function of fluidity $1/\eta$ of a helix with a 30 nm helical radius, $L/R = 5.92$ pitch length and helical radius ratio, and $N = 1.25$ helical turns. The lines are linear fits to the data without thermal fluctuations.

## Péclet number

To quantify the influence of the external torque on the directed motion of the helices, we calculate the Péclet number that is defined as the ratio of the diffusive and the advective time scales. For our system, the Péclet number is given by $\mathrm{Pe} = vL/D_T$, where $v$ is the propulsion velocity, $L$ is the length of the helix, and $D_T$ is the tracer diffusion coefficient of the particle (see SI Figs. 9 and 10). The propulsion velocity used in the calculation of the Péclet number is the propulsion velocity obtained in the absence of the thermal fluctuations in the fluid. The diffusion coefficient $D_T = k_B T/\gamma$ was obtained by measuring the effective drag coefficients $\gamma$ of the stationary helical particles in Poiseuille flow. The effective drag coefficients depend on the orientation of the helix with the fluid flow through the relation $1/\gamma = (1/\gamma_\perp + 2/\gamma_\parallel)/3$.

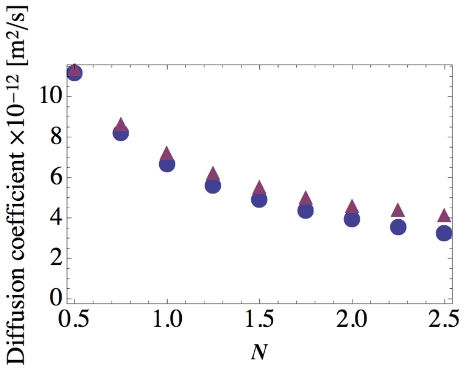


Figure S9: Diffusion coefficients (DCs) as a function of the number of turns of a helix with a 30 nm helical radius, and $L/R = 5.92$ pitch length and helical radius ratio. Circles and triangles are the DCs for motion along the parallel and perpendicular axis of the helix. The DC for motion along the parallel is inversely proportional to the length of the helix.

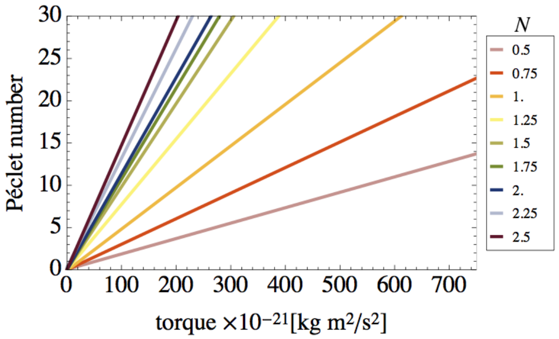


(a)

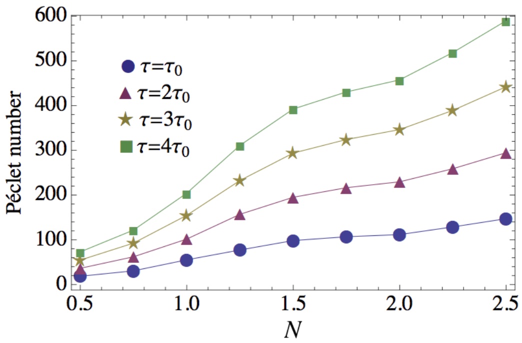


(b)

Figure S10: a. Péclet number as a function of the number of helical turns for helices with a pitch length to helical radius ratio of $L/R = 5.92$ and a varying external torque in a fluid at temperature $T = 300$ K. b. Péclet numbers of a helix of pitch length to helical radius ratio of $L/R = 5.92$ with varying number of helical turns as a function of the applied external torque. Here, $\tau_0 = 10^{-18}$ kg m$^2$/s$^2$.

# Chiral separation

Fig. 4 in the main text shows the chiral separation of (+) and (−) helices in the presence of thermal fluctuations; Fig. S11 shows the trajectories of (+) and (−) helices without thermal fluctuations and with the same driving torques in Fig. 4.

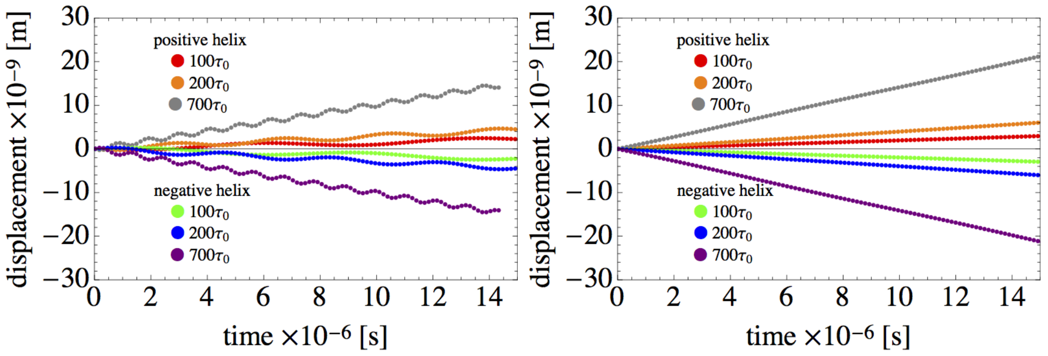


(a) $N = 0.5$

(b) $N = 1.25$

Figure S11: Deterministic displacements along the $\hat{u}_x$-direction of (+) and (−) helices with (a) $N = 0.5$ and (b) $N = 1.25$ turns that are driven by varying constant external torques without thermal fluctuations. $\tau_0 = 10^{-21}$ kg m$^2$/s$^2$.

# Finite size effects

An important aspect of any hydrodynamic simulations is a careful consideration of the finite-size effects due to the long range of fluid-mediated hydrodynamic interactions between the particle and its images due to the periodic boundary conditions. We have examined them here by simulating the propulsion of helices and helicoids in a viscous fluid in the absence of thermal fluctuations. We have first verified that for the system sizes considered here, finite-size effects for the angular velocities of the helices are negligible. However, for the calculation of the propulsion velocities they have to be taken into account. In Ref. 1 there is an analytical solution to the Stokes equations of motion for a viscous fluid flowing past spatially periodic obstacles. To first order, the drag force experienced by an obstacle is proportional to the fluid flow velocity based on the relation

$$F_{\mathrm{drag}} = \frac{6\pi\eta R_H v}{1 - \frac{B}{\mathcal{L}} R_H} \tag{2}$$

where $R_H$ is the effective hydrodynamic size of the particle and $\mathcal{L}$ is the distance between the points of the cubic lattice [1]. The constant $B$ for a simple cubic geometry is $B = 2.8373$. This analytical approximation for the dependence of the drag coefficient on system size has been found to be in excellent agreement with numerical simulations of the diffusion of colloidal particles [2, 3]. The measured propulsion velocity for varying system size is fitted to equation (2) and the velocity is extrapolated for $\mathcal{L} \to \infty$ by treating the drag force and the effective hydrodynamic size of the particle as free parameters. In Figure 12, the propulsion velocity of a 30 nm helical particle with $L/R = 5.92$ and a length of 177 nm is plotted against the system size $\mathcal{L}$. The extrapolated value of the propulsion velocity for $\tau = 1.0 \times 10^{-18}$ kg m$^2$/s obtained using the modified Stokes equation of motion (Equation (2)) is $(1.63 \pm 0.01) \times 10^{-3}$ nm/ns. The maximum deviation of the measured propulsion velocity for the system sizes tested from the extrapolated propulsion velocity is 2.8%.

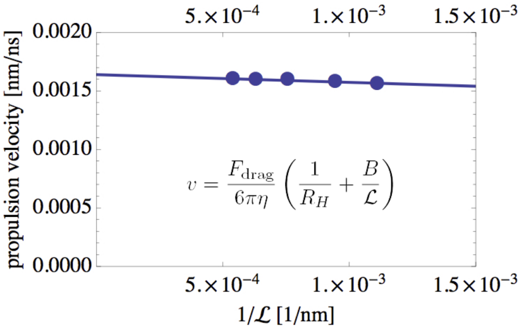


Figure S12: Propulsion velocity of a 30 nm helical particle with $N = 1.25$ helical turns as a function of the system size, $\mathcal{L}$. The solid line is an analytical fit to the finite size effects for the propulsion velocity where $a$ is the effective size of the helical particle and $B = 2.8373$.

# References

[1] H Hasimoto. On the periodic fundamental solutions of the stokes equations and their application to viscous flow past a cubic array of spheres. *J. Fluid Mech.*, 5(02), 1959.

[2] Santtu T T Ollila, Colin Denniston, Mikko Karttunen, and Tapio Ala-Nissila. Fluctuating lattice-Boltzmann model for complex fluids. *J. Chem. Phys.*, 134(6):064902, February 2011.

[3] In-Chul Yeh and Gerhard Hummer. System-Size Dependence of Diffusion Coefficients and Viscosities from Molecular Dynamics Simulations with Periodic Boundary Conditions. *J. Phys. Chem. B*, 108(40):15873–15879, October 2004.
